# Supplementary material for: Can experimentally-accessible measures of entanglement distinguish quantum spin liquids from disorder-driven "random singlet" phases ?
Source: arXiv:2505.11874 source file (2025-05-17)
Supplement: Supplementary file 1 [file supple.pdf]

# Can experimentally-accessible measures of entanglement distinguish quantum spin liquids from disorder–driven "random singlet" phases ?
# -Supplementary information-

Tokuro Shimokawa,[1,*] Snigdh Sabharwal,[1] and Nic Shannon[1]

[1]*Theory of Quantum Matter Unit, Okinawa Institute of Science and Technology Graduate University, Onna-son, Okinawa 904-0412, Japan*

(Dated: May 17, 2025)

## I. EXACT DIAGONALIZATION CALCULATIONS AT $T = 0$

The calculations of entanglement measures at $T = 0$, presented in Fig. 1 and Fig 3 of the main text, were carried out using conventional exact diagonalization (ED) methods. Within these, the Hamiltonian

$$\mathcal{H} = J_1 \sum_{\langle ij \rangle_1} (1 + \Delta\alpha_{ij}) \mathbf{S}_i \cdot \mathbf{S}_j + J_2 \sum_{\langle ij \rangle_2} (1 + \Delta\beta_{ij}) \mathbf{S}_i \cdot \mathbf{S}_j \ ,$$
$$\alpha_{ij}, \beta_{ij} \in [-1, 1] \ , \quad \text{(S1)}$$

was solved on a finite cluster of size

$$N \in \{18, 24, 24, 30\} \ , \quad \text{(S2)}$$

subject periodic boundary conditions, using a standard Lanczos algorithm, implemented through a modified version of TITPACK ver. 2 [1]. The geometries of the clusters considered is illustrated in Fig. S1.

Physical properties in the presence of disorder [$\Delta \neq 0$], were estimated by taking an average within $M_{\mathsf{N}}$ different realizations of bond–disorder $\{J_{ij}\}$, chosen from the ensemble defined in Eq. (S1). These averages were calculated as

$$\overline{\langle \hat{A} \rangle} = \frac{1}{M_{\mathsf{N}}} \sum_{m=0}^{M_{\mathsf{N}}-1} \langle \hat{A} \rangle^{(m)} \ , \quad \text{(S3)}$$

where $\langle \hat{A} \rangle^{(m)}$ represents the expectation of value of an operator $\hat{A}$ within the $m^{\text{th}}$ realization of disorder, calculated using ED at $T = 0$, and quantum typicality methods for $T > 0$, as described below. In calculations, this average was typically calculated over

$$M_{\mathsf{N}} \sim 80 \qquad [N = 18] \ , \quad \text{(S4a)}$$
$$M_{\mathsf{N}} \sim 40 \qquad [N = 24] \ , \quad \text{(S4b)}$$
$$M_{\mathsf{N}} \sim 20 \qquad [N = 30] \ , \quad \text{(S4c)}$$

realizations of disorder.

The model, Eq. (S1) supports four different ground states as a function of $(J_1, J_2, \Delta)$: three–sublattice Néel order; a quantum spin liquid (QSL); stripe–like order; and a disorder–driven "random singlet" (RS) phase [cf. Fig. 2 of the main text]. The Néel, QSL and RS phases all exhibit two–point correlations which are peaked at the three–sublattice wave vector

$$\mathbf{q}_{\mathsf{K}} = \left( \frac{4\pi}{3}, 0 \right) \ , \quad \text{(S5)}$$

* tokuro.shimokawa@oist.jp

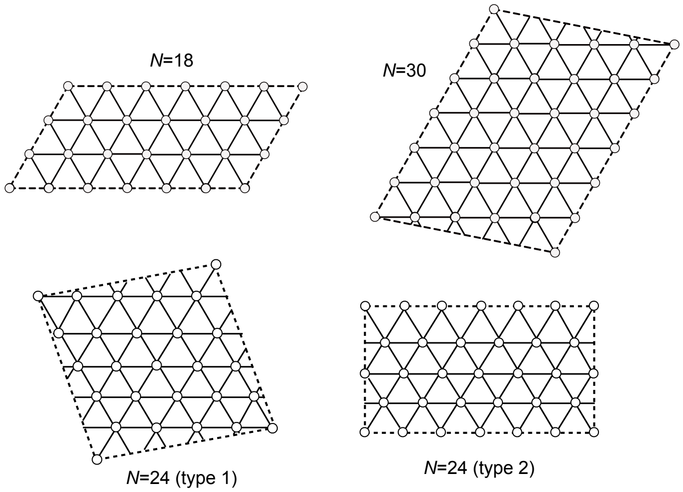


Figure S1. Finite–size clusters used in numerical calculations. Periodic boundary conditions equivalent to a taurus were imposed, with the periodic boundaries illustrated through dashed lines.

(and symmetry–related wavectors), as revealed by the equal time structure factor

$$S(\mathbf{q}) = \frac{1}{N} \langle | \sum_i \mathbf{S}_j e^{i\mathbf{q}\cdot\mathbf{r}_i} |^2 \rangle \ , \quad \text{(S6)}$$

calculated for parameters

$$(J_1, J_2, \Delta) = (1, 0, 0) \qquad [\text{Néel}] \quad \text{(S7a)}$$
$$(J_1, J_2, \Delta) = (1, 0.12, 0) \qquad [\text{QSL}] \quad \text{(S7b)}$$
$$(J_1, J_2, \Delta) = (1, 0, 1) \qquad [\text{RS}] \quad \text{(S7c)}$$

and illustrated in Fig. S2.

## II. DETERMINATION OF $T = 0$ PHASE TRANSITIONS THROUGH ENTANGLEMENT WITNESSES

In the main text we have argued that there are qualitative differences in concurrence (and thereby two–tangle) which distinguish quantum spin liquid (QSL) from disorder–driven "random singlet" (RS) phases [cf. Fig 1, Fig. 3 of main text]. Here we show how two different measures of entanglement, the one–tangle and two–tangle, can be used to identify the zero–temperature phase transition from Néel to RS phases as a function of disorder, in simulations of the triangular lattice model, Eq (S1).

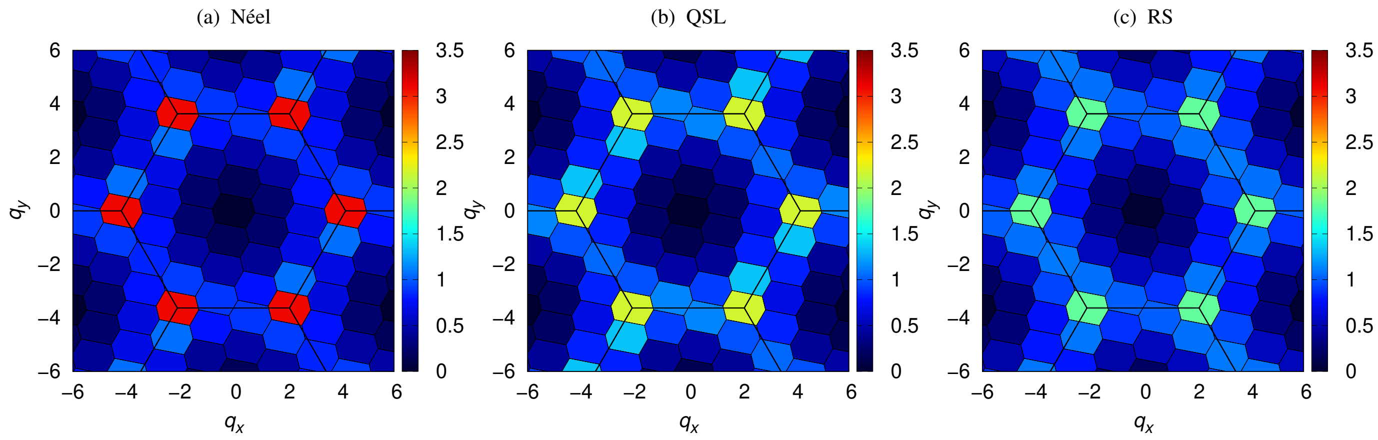


Figure S2. Comparison of correlations in Néel, quantum spin liquid (QSL) and disorder–driven "random singlet" (RS) phases, showing dominant role of fluctuations at the K–point in reciprocal space. (a) Results for equal time structure factor $S(\mathbf{q})$ [Eq. (S6)] within Néel phase, showing Bragg peaks at the three–sublattice wavevector $\mathbf{q}_{\mathsf{K}}$ [Eq. (S5)]. (b) Equivalent results for QSL, showing correlations centered on zone boundary, with maxima at $\mathbf{q}_{\mathsf{K}}$. (c) Equivalent results for RS phase, showing diffuse correlations with maxima at $\mathbf{q}_{\mathsf{K}}$. Results were obtained with $T = 0$ exact diagonalization (ED) calculations for the disordered triangular–lattice model, Eq. (S1), on a cluster of $N = 30$ spins [Fig. S1], with parameters Eq. (S7).

The one–tangle

$$\tau_j^{(1)} = 1 - 4\langle S_j^z \rangle^2 . \tag{S8}$$

provides a measure of the extent to which a single spin in a quantum spin system is entangled with other spins, under the assumption that the system has (at least) a $U(1)$ symmetry [2–4]. The entanglement measured by one–tangle may occur at any depth, i.e. involve pairs of spin, triples of spins, etc. We consider both averages of $\tau^{(1)}$ within different realizations of bond disorder

$$\overline{\tau^{(1)}} = \frac{1}{M_{\mathsf{N}}} \sum_{m=0}^{M_{\mathsf{N}}-1} \langle \tau_j^{(1)} \rangle^{(m)} , \tag{S9}$$

and the one–tangle evaluated for correlations within a disordered state

$$\tilde{\tau}^{(1)} = 1 - 4\overline{\langle S_j^z \rangle}^2 , \tag{S10}$$

as measured in experiment.

Meanwhile the two–tangle

$$\tau_j^{(2)} = \sum_{i \neq j} C_{ij}^2 , \tag{S11}$$

is derived from concurrence,

$$C_{ij} = 2\max\{0, \sqrt{\left(\langle S_i^x S_j^x \rangle + \langle S_i^y S_j^y \rangle\right)^2} - \sqrt{\left(\frac{1}{4} + \langle S_i^z S_j^z \rangle\right)^2 - \left(\frac{\langle S_i^z \rangle + \langle S_j^z \rangle}{2}\right)^2}\} , \tag{S12}$$

and quantifies the amount of this entanglement which associated with pairs of spins, again under the assumption that the system has (at least) a $U(1)$ symmetry [2–4]. We consider both the average of $\tau^{(2)}$ within different realizations of bond disorder

$$\overline{\tau^{(2)}} = \frac{1}{M_{\mathsf{N}}} \sum_{m=0}^{M_{\mathsf{N}}-1} \langle \tau_j^{(2)} \rangle^{(m)} , \tag{S13}$$

and the two–tangle evaluated for correlations within a disordered state, as measured in experiment

$$\tilde{\tau}^{(2)} = \sum_{i \neq j} \tilde{C}_{ij}^2 , \tag{S14}$$

where

$$\tilde{C}_{ij} = 2\max\{0, \sqrt{(\overline{\langle S_i^x S_j^x \rangle} + \overline{\langle S_i^y S_j^y \rangle})^2} - \sqrt{\left(\frac{1}{4} + \overline{\langle S_i^z S_j^z \rangle}\right)^2 - \left(\frac{\overline{\langle S_i^z \rangle} + \overline{\langle S_j^z \rangle}}{2}\right)^2}\}. \tag{S15}$$

In Fig. S3 we show how disorder averages of the one–tangle and two–tangle evolve in the ground state of Eq (S1), within exact diagonalization (ED) calculations carried out for clusters of size $N = 12 \ldots 30$ [Fig. S1], with parameters

$$(J_1, J_2, \Delta) = (1, 0, \Delta) . \tag{S16}$$

Earlier work on this model [5, 6], identified a phase transition from three–sublattice Néel to RS phases, occurring for $\Delta \lesssim 0.6$ [cf. phase diagram, Fig. 2 of main text]. This phase boundary was determined through an analysis of thermodynamic quantities [5, 6], supplemented by entanglement spectra [6].

We find that the one–tangle, $\overline{\tau^{(1)}}$ [Eq. (S9)], is weakly sensitive to the phase transition from Néel to RS ground states. In the Néel ground state, for $\Delta \lesssim 0.6$, we find $\overline{\tau^{(1)}} \equiv 1$, reflecting the fact that ground state of a finite–size cluster is a singlet,

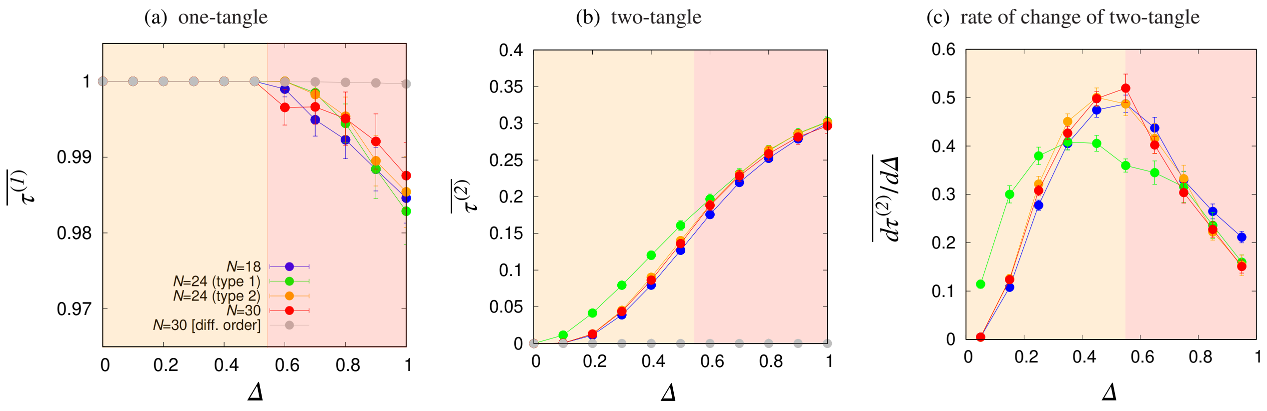


Figure S3. Determination of a zero–temperature phase transition from entanglement witnesses. (a) Dependence of the one–tangle $\overline{\tau^{(1)}}$ [Eq. (S9)] on disorder $\Delta$, demonstrating sensitivity to the phase transition from Néel to disorder driven random singlet (RS) phases at $\Delta \approx 0.6$. When disorder averages are taken in order relevant to experiment [Eq. (S10), grey points], sensitivity to the phase transition is lost. (b) Two–tangle $\overline{\tau^{(2)}}$ [Eq. (S13)], showing evolution of two–spin entanglement as a function of disorder, $\Delta$. The phase transition from Néel to RS ground states is distinguished by a point of inflection. When disorder averages are taken in order relevant to experiment [Eq. (S14), grey points], all sensitivity to two–spin entanglement is lost [8]. (c) First derivative of $\overline{\tau^{(2)}}$ with respect to $\Delta$, exhibiting a maximum at the phase transition from Néel to RS ground states. Results are shown for exact diagonalization calculations of ground states of Eq. (S1), with parameters Eq. (S16).

with total spin $S = 0$, and cannot break spin–rotation symmetry. Within this Néel ground state, individual spins are both strongly, and deeply, entangled. Meanwhile in the RS ground state, for $\Delta \gtrsim 0.6$, $\overline{\tau^{(1)}}$ starts to deviate from 1, tending to a value $\overline{\tau^{(1)}} \sim 0.99$ for $\Delta \to 1$ [Fig. (S3a)]. We attribute this small reduction in the one–tangle to the existence of ground states with a finite total spin, and thereby a finite $S^z$, for some realizations of disorder, as previously discussed in [7]. Once the disorder averages is taken in order measured in experiment, $\tilde{\tau}^{(1)}$ [Eq. (S10)], the contributions of these states sums to zero, and the one–tangle loses all sensitivity to the phase transition from Néel to RS ground states. Results for $\tilde{\tau}^{(1)}$ are shown with grey circles in Fig. (S3a).

A more discriminating probe of the transition from Néel to RS phases is provided by the two–tangle $\overline{\tau^{(2)}}$ [Eq. (S13)], shown in Fig. S3b. This is exhibits a point of inflection at the phase transition, $\Delta \approx 0.6$. But once again, if averages are taken in the order relevant to experiment, $\tilde{\tau}^{(2)}$ [Eq. (S14), grey points], all sensitivity to two–spin entanglement is lost. The point of inflection in the two–tangle can identified more easily if the derivative of $\overline{\tau^{(2)}}$ is taken with respect to $\Delta$. This is illustrated in Fig. S3c.

From these results, we learn three things:

1. That measuring changes in one– and two–tangle provide a practical strategy for identifying the phase transitions into the RS phase, in simulation.

2. That measuring changes in one– and two–tangle *do not* provide a practical strategy for identifying the phase transitions into the RS phase in experiment.

3. That the RS ground state exhibits many–partite entanglement [cf. Ref. 8].

This last results follows from the fact that the two–partite entanglement measured by the two–tangle in the RS phase $\overline{\tau^{(2)}} \sim 0.2$—$0.3$ does not saturate the entanglement witnessed by the one–tangle $\overline{\tau^{(1)}} \approx 1$ [2].

## III. QUANTUM TYPICALITY CALCULATIONS

The direct application of exact diagonalization (ED) to quantum states at finite temperature requires a complete enumeration of states, and so is extremely memory-intensive, restricting systems sizes to $N \sim 20$ spins for $S = 1/2$ systems. In this study, we have instead employed a quantum typicality method, namely, based on thermal pure quantum (TPQ) states, also known as the Hams-de Raedt method [9–15]. This approach allows the calculation of physical properties by focusing on a limited set of quantum states rather than averaging over the entire Hilbert space. As a result, it is possible to calculate thermodynamic and dynamical properties at finite temperature with high accuracy, for clusters of up to $N \sim 40$ spins. In the present study, where we address dynamical properties in the presence of disorder, calculations were carried out for clusters of $N \leq 30$ spins. These were defined on torus with periodic boundary conditions, as illustrated in Fig. S1. In what follows, we briefly outline the essentials of the TPQ method.

The TPQ approach is based on the construction of a ensemble of thermal pure states, within which it is possible to calcuate both quantum and thermal averages. We consider a system of size $N$, with Hilbert space dimension $D$, described by a Hamilonian $\mathcal{H}$, at inverse temperature

$$\beta = 1/T \; . \tag{S17}$$

States

$$|\beta, N\rangle = e^{-\beta\mathcal{H}/2}|\psi_0\rangle \; , \tag{S18}$$

are constructed from initial vectors

$$|\psi_0\rangle = \sum_i^D c_i |i\rangle \ , \tag{S19}$$

where the coefficients $c_i$ are complex numbers, chosen at random, which satisfy the normalization condition

$$\sum_i |c_i|^2 = 1 \ . \tag{S20}$$

As such, $\{|i\rangle\}$ form an arbitrary orthonormal basis for the Hilbert space of the target Hamiltonian $\mathcal{H}$.

Within the TPQ approach, thermal expectation values of operators are estimated as averages $\overline{\langle \ldots \rangle}$ over $I_{\mathsf{N}}$ initial states chosen from this ensemble

$$\langle \hat{A} \rangle = \frac{\overline{\langle \beta, N | \hat{A} | \beta, N \rangle}}{\overline{\langle \beta, N | \beta, N \rangle}} \ . \tag{S21}$$

The deviation of this estimator from the true expectation value can be shown to scale as

$$\Delta \langle \hat{A} \rangle \sim 1/\sqrt{I_{\mathsf{N}} D} \tag{S22}$$

[10]. As consequence, for a large system, accurate estimates can be obtained from a relatively small number of initial random states. In cases where the (thermal) entropy remains large at the temperatures considered, a condition commonly satisfied in frustrated systems, the number of initial vectors needed to obtain accurate estimates is particularly small [13]. In the example considered here, we find

$$I_{\mathsf{N}} \lesssim \mathcal{O}(10) \tag{S23}$$

is sufficient to obtain well–converged estimates.

Estimates of the dynamical structure $S(\mathbf{q}, \omega, T)$ factor can be constructed within this ensemble of thermal states, by evaluating the (real) time evolution of correlations [14]. We consider

$$\langle S^z_{-\mathbf{q}}(t=0) S^z_{\mathbf{q}}(t) \rangle = \langle \beta, N | S^z_{-\mathbf{q}} e^{i\mathcal{H}t} S^z_{\mathbf{q}} e^{-i\mathcal{H}t} | \beta, N \rangle, \tag{S24}$$

where

$$S^z_{\mathbf{q}} = \frac{1}{\sqrt{N}} \sum_j S^z_i e^{i\mathbf{q}\cdot\mathbf{r}_i} \ , \tag{S25}$$

and construct the vectors

$$|A(t)\rangle \equiv e^{-i\mathcal{H}t} |\beta, N\rangle \ , \tag{S26}$$

and

$$|B(t)\rangle \equiv e^{-i\mathcal{H}t} S^z_{\mathbf{q}} |\beta, N\rangle \ . \tag{S27}$$

The time–dependence of $|A(t)\rangle$ and $|B(t)\rangle$ depends on the operator $e^{-i\mathcal{H}t}$, which we resolve using a Chebyshev polynomial expansion [16]

$$e^{-i\mathcal{H}t} |\beta, N\rangle = e^{-it\bar{\lambda}} \{ J_0(\tau) + 2 i^k \sum_{k=1}^m J_k(\tau) T_k(-\mathcal{H}_{\rm sc}) \} |\beta, N\rangle \ , \tag{S28}$$

where

$$\bar{\lambda} = \frac{1}{2}(E_{\rm max} + E_{\rm min}) \ , \tag{S29}$$

and

$$\delta\lambda = \frac{1}{2}(E_{\rm max} - E_{\rm min}) \ , \tag{S30}$$

are characteristic energy scales set by the maximal and minimal eigenvalues of the target Hamiltonian

$$\mathcal{H} |E_{\rm max}\rangle = E_{\rm max} |E_{\rm max}\rangle \ , \text{ etc. } ; \tag{S31}$$

$J_k(\tau)$ is a Bessel function of the first kind;

$$\tau = \delta\lambda \, t \ , \tag{S32}$$

a reduced time; and $T_k(-\mathcal{H}_{\rm sc})$ is the $k$-th order Chebyshev polynomial associated with the renormalized Hamiltonian

$$\mathcal{H}_{\rm sc} = \frac{\mathcal{H} - \bar{\lambda}}{\delta\lambda} \ . \tag{S33}$$

The integer $m$ in Eq. (S28) determines the order of the expansion, and is taken to be sufficiently large to ensure the convergence of results. Values of $E_{\rm max}$ and $E_{\rm min}$ can be found through a standard Lanczos calculation for the target Hamiltonian $\mathcal{H}$.

We determine $S^{zz}(\mathbf{q}, t, T)$ [Eq. (S24)] by constructing a discrete time series

$$\{t_i\} = \{0, \ \delta t, \ 2\delta t, \ \ldots, \ t_{\rm max}\} \ , \tag{S34}$$

and evaluating

$$\langle B(t_i) | S^z_{\mathbf{q}} | A(t_i) \rangle \tag{S35}$$

through Eq. (S26) and Eq. (S27), to obtain estimates for

$$S^{zz}(\mathbf{q}, t_i, T) \quad \forall \quad t \in \{t_i\} \tag{S36}$$

Given these results, the dynamical structure factor as function of $\omega$ can be obtained through discrete Fourier transformation

$$S^{zz}(\mathbf{q}, \omega, T) = \frac{\delta t}{\pi} \sum_{t_i > 0} \frac{\mathrm{Re}[\overline{\langle S^z_{-\mathbf{q}}(0) S^z_{\mathbf{q}}(t_i) \rangle} e^{-i\omega t_i}]}{\overline{\langle \beta, N | \beta, N \rangle}} \times e^{-\frac{1}{2}(\gamma \frac{t_i}{t_{\rm max}})^2} + \frac{\delta t}{2\pi} \frac{\overline{\langle S^z_{-\mathbf{q}}(0) S^z_{\mathbf{q}}(0) \rangle}}{\overline{\langle \beta, N | \beta, N \rangle}} \tag{S37}$$

A Gaussian window function with

$$\gamma = 5.0 \tag{S38}$$

is included to mitigate Gibbs oscillations [14]. The expectation values $\overline{\langle \ldots \rangle}$ are calculated using $I_{\mathsf{N}}$ initial vectors

$$I_{\mathsf{N}} \sim 20 \qquad [N = 18] \ , \tag{S39a}$$

$$I_{\mathsf{N}} \sim 10 \qquad [N = 24] \ , \tag{S39b}$$

$$I_{\mathsf{N}} \sim \ \ 4 \qquad [N = 30] \ , \tag{S39c}$$

following Eq. (S21), and further averaged over $M$ different realizations of disorder, following Eq. (S13) and Eq. (S4).

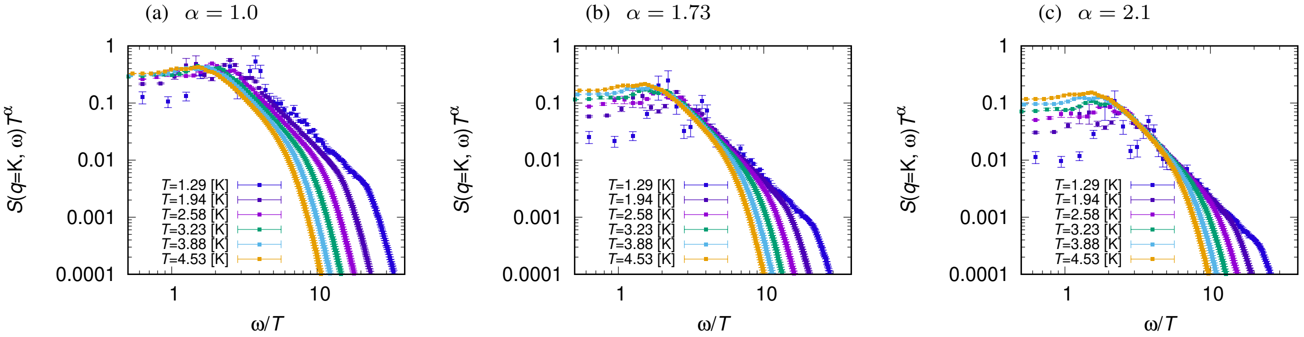


Figure S4. Scaling collapse of dynamical structure factor found in simulations of a triangular lattice antiferromagnet, as function of critical exponent, $\alpha$. In all cases, data is scaled according to Eq. (S42). (a) Scaling for the value of exponent predicted by spin wave theory, $\alpha = 1.0$, showing the failure of data to collapse onto a single curve. (b) Scaling for the exponent found in experiment, $\alpha = 1.73$ [17], showing a satisfactory collapse of simulation results. (c) Scaling for exponent $\alpha = 2.1$, showing a marginally better collapse of simulation results. Results are taken from quantum typicality calculations of $S^{zz}(\mathbf{q}, \omega)$ [Eq. S37], for the minimal model of $KYSe_2$ [Eq. S1], with parameters taken from experiment, Eq. (S41).

We note that the duration of simulations, $t_{\rm max}$, places a bound the energy resolution which can be achieved in simulation, while the time–step, $\delta t$, determines the highest frequency which can be addressed. For the problem considered, we find

$$\delta t = 0.05 \sim 0.1 \ J_1^{-1} \ , \quad \text{(S40a)}$$

$$t_{\rm max} = 80 \sim 100 \ J_1^{-1} \ . \quad \text{(S40b)}$$

provides sufficient accuracy.

## IV. DYNAMICAL SCALING OF SIMULATION RESULTS

As shown in Fig. 5 of the main text, both experimental data for $KYbSe_2$ [17], and simulation results for the model Eq. (S1) with parameters taken from experiment

$$(J_1, J_2, \Delta) = (1, 0.047, 0) \qquad [\mathrm{KYbSe_2}] \ , \quad \text{(S41)}$$

exhibit a scaling collapse of the dynamical structure factor $S(\mathbf{q}_{\mathsf{K}}, \omega, T)$, of the form

$$T^\alpha S(\mathbf{q}_{\mathsf{K}}, \omega, T) = \Phi\left(\frac{\hbar\omega}{k_B T}\right) \ , \quad \text{(S42)}$$

with exponent $\alpha = 1.73$.

In Fig. S4 we explore how this scaling collapse depends on the value of exponent $\alpha$. In Fig. S4a results are shown for the value of exponent predicted by spin wave theory, $\alpha = 1.0$ [17]. For this value of exponent, data fail to collapse onto a single curve, suggesting that spin wave theory provides a poor account of dynamics over this range of $\omega/T$. In contrast, the value of exponent found in experiment, $\alpha = 1.73$, leads a satisfactory collapse of simulation data over the accessible range of $\omega/T$, as shown in Fig. S4b [cf. Fig. 5(e) of the main text].

The optimal collapse of simulation data over this range of $\omega/T$ is found for $\alpha = 2.1$. This is illustrated in Fig. S4c. However the collapse of data for $\alpha = 2.1$ is only marginally better than that obtained for $\alpha = 1.73$, suggesting that results for a greater range of $\omega/T$ would be needed to make a definitive estimate of the exponent $\alpha$. Since the range of $\omega/T$ available in published INS data [17] is similar to that available in simulation, this may also be true for experiment.

Not withstanding, some difference in the value of $\alpha$ found in experiment and simulation might be anticipated, since the spin–rotational invariant model, Eq. (S1), is at best an approximation to anisotropic exchange interactions between $Yb^{3+}$ ions [18]. Moreover, the fact that a scaling collapse can be obtained for a non–trivial exponent $\alpha \approx 2$ remains a striking feature of both experiment and simulation. This scaling collapse lends weight to the idea that both model [19] and material [17] lie close in parameter space to a quantum critical point.

[1] H. Nishimori, TITPACK ver. 2. (2023).
[2] V. Coffman, J. Kundu, and W. K. Wootters, Phys. Rev. A **61**, 052306 (2000).
[3] L. Amico, A. Osterloh, F. Plastina, R. Fazio, and G. Massimo Palma, Phys. Rev. A **69**, 022304 (2004).
[4] L. Amico, F. Baroni, A. Fubini, D. Patanè, V. Tognetti, and P. Verrucchi, Phys. Rev. A **74**, 022322 (2006).
[5] K. Watanabe, H. Kawamura, H. Nakano, and T. Sakai, Journal of the Physical Society of Japan **83**, 034714 (2014), https://doi.org/10.7566/JPSJ.83.034714.
[6] H.-Q. Wu, S.-S. Gong, and D. N. Sheng, Phys. Rev. B **99**, 085141 (2019).
[7] H. Kawamura and K. Uematsu, Journal of Physics: Condensed Matter **31**, 504003 (2019).
[8] S. Sabharwal, T. Shimokawa, and N. Shannon, "Witnessing disorder in quantum magnets," Accepted for publication in PRResearch (2024), arXiv:2407.20797 [cond-mat.str-el].
[9] M. Imada and M. Takahashi, Journal of the Physical Society of

Japan **55**, 3354 (1986), https://doi.org/10.1143/JPSJ.55.3354.
[10] A. Hams and H. De Raedt, Phys. Rev. E **62**, 4365 (2000).
[11] T. Iitaka and T. Ebisuzaki, Phys. Rev. Lett. **90**, 047203 (2003).
[12] M. Machida, T. Iitaka, and S. Miyashita, Phys. Rev. B **86**, 224412 (2012).
[13] S. Sugiura and A. Shimizu, Phys. Rev. Lett. **111**, 010401 (2013).
[14] H. Ikeuchi, H. De Raedt, S. Bertaina, and S. Miyashita, Phys. Rev. B **92**, 214431 (2015).
[15] H. Endo, C. Hotta, and A. Shimizu, Phys. Rev. Lett. **121**, 220601 (2018).
[16] W. H. Press, S. A. Teukolsky, W. T. Vetterling, and B. P. Flannery, Numerical Recipes: The Art of Scientific Computing (Third Edition) (Cambridge University Press, 2007).
[17] A. O. Scheie, E. A. Ghioldi, J. Xing, J. A. M. Paddison, N. E. Sherman, M. Dupont, L. D. Sanjeewa, S. Lee, A. J. Woods, D. Abernathy, D. M. Pajerowski, T. J. Williams, S.-S. Zhang, L. O. Manuel, A. E. Trumper, C. D. Pemmaraju, A. S. Sefat, D. S. Parker, T. P. Devereaux, R. Movshovich, J. E. Moore, C. D. Batista, and D. A. Tennant, Nature Physics **20**, 74 (2024).
[18] Z. Zhu, P. A. Maksimov, S. R. White, and A. L. Chernyshev, Phys. Rev. Lett. **119**, 157201 (2017).
[19] R. Kaneko, S. Morita, and M. Imada, Journal of the Physical Society of Japan **83**, 093707 (2014), https://doi.org/10.7566/JPSJ.83.093707.
